# Supplementary material for: PopIns: population-scale detection of novel sequence insertions
Source: arXiv:1504.01813 source file (2015-04-08)
Supplement: Supplementary file 1 [file supplement.pdf]

# Supplementary material to “PopIns: population-scale detection of novel sequence insertions”

Birte Kehr [1,*], Páll Melsted [1,2] and Bjarni V. Halldórsson [1,3]

[1]deCODE genetics/Amgen, Reykjavík, Iceland
[2]Faculty of Industrial Engineering, Mechanical Engineering and Computer Science, University of Iceland, Reykjavík, Iceland
[3]Institute of Biomedical and Neural Engineering, Reykjavík University, Reykjavík, Iceland

## S1 Method details

### S1.1 Choice of assembly program and parameters

The assembly program and its parameters were chosen by comparing the contigs output by three different assemblers, *Velvet* (?), *MaSuRCA* (?), and *SPAdes* (?). Additionally, *Velvet* was run using three $k$-mer values, $31, 47$, and 63. *SPAdes* and *MaSuRCA* were run with default parameters and *Velvet* was configured to remove low and high coverage contigs with a coverage window of $[2, 100]$. Of the assemblers, *Velvet* has arguably the simplest algorithm for building a de Bruijn graph, removing errors and resolving repeats using paired end reads. *SPAdes* uses a similar paradigm, but builds de Bruijn graphs for several values of $k$, by default $21, 33$, and 55 and combines the assemblies in an iterative fashion. Additionally *SPAdes* uses paired end reads to resolve repetitive regions using paired de Bruijn graphs (?). *MaSuRCA* is a hybrid of regular de Bruijn graph construction and Overlap-Layout-Consensus approaches by using the de Bruijn graphs to construct super reads used in the OLC approach.

The two key elements that affect the assembly are the parameters used, most importantly $k$-mer size, and the implicit assumptions the assembler makes when simplifying the assembly. Most assemblers are made for whole genome assembly, and the simplifications they make when correcting for errors or resolving repetitive regions are usually based on this premise. Since the reads used for contig construction are not sampled from the whole genome, but rather from several disjoint locations in the genome, this can result in suboptimal contig construction. The choice of $k$ involves a tradeoff between quality and quantity. For larger values of $k$ the assembler has an easier task of resolving low complexity regions as the $k$-mers tend to be more unique. However with large $k$ the effect of sequencing errors becomes more evident as it reduces the coverage of $k$-mers, thus resulting in missed connections and a more fragmented assembly.

Based on these observations we compared the five assembly methods by generating contigs for a single individual, whose sequencing coverage value of $23\times$ coverage was the median over all the individuals. Table S1 shows the statistics for the assemblies generated. To compare overlap between the assemblies, the contigs generated for each method were pairwisely aligned using *Stellar* (?) with a minimum alignment length of 50 bp and a maximum of 2% errors.

Based on the sum of basepairs of all the contigs, we eliminated the *MaSuRCA* output from consideration (this short output is most likely because *MaSuRCA* is made for whole genome assembly, rather than individual contig assembly). Next we looked at the *Velvet* ($k = 63$) output. Most likely, the large value for $k$ resulted in too low coverage and a shorter output. When aligning the contigs of *Velvet* ($k = 63$) 95-98 % of the basepairs matched to the contigs of the remaining assemblies. *Velvet* ($k = 31$) generated the most output, but also the lowest N50 value, indicating that the additional contigs assembled are relatively short. For instance compared to *Velvet* ($k = 47$), the $k = 31$ contains 93 % of the basepairs of $k = 47$ whereas $k = 47$

[*]to whom correspondence should be addressed

contains 71 % of the basepairs of $k = 31$. Finally comparing the output of *SPAdes* and *Velvet* ($k = 47$) we note that *Velvet* generates more contigs at the expense of a lower N50. The overlap percentage of *Velvet* contigs contained in *SPAdes* is 83 %, and 88 % of *SPAdes* contained in the *Velvet* output. Given the similar contig values and high overlap we opted for using *Velvet* with $k = 47$ since the assembly process was quicker and *Velvet* has a simpler assembly algorithm.

## S1.2 Merging

### S1.2.1 Partitioning contigs into sets.

As in the main text, let $C_1, \ldots, C_n$ be the sets of contigs from $n$ individuals and $\mathcal{C} = \bigcup_i C_i$. In order to add a contig $c \in \mathcal{C}$ to a union-find instance $\mathcal{D}$, we take the union of all sets in $\mathcal{D}$ that contain at least one contig that locally aligns to $c$. In addition, we add $c$ to this union. If $c$ aligns to none of the contigs previously added to $\mathcal{D}$, we add a new set containing only $c$.

In the worst case, our partitioning strategy requires local alignment computations for all pairs of the contigs in $\mathcal{C}$. Given the number of individuals and number of contigs per individual, we cannot afford to use standard dynamic programming on all pairs of contigs. Instead, we filter for local similarity using *SWIFT* and only verify a significant local alignment using dynamic programming when two sequences pass the *SWIFT* filter. Furthermore, we skip verification by dynamic programming if two contigs are already known to be elements of the same set. For each set, we further keep track of the pairs of contigs $\mathcal{V}$, where the local alignment has been verified.

We can consider the contigs to be nodes in a graph with an edge between the nodes of any two contigs that have a local alignment. In this graph, the sets $D_1, \ldots, D_k$ correspond to connected components. In practice, we expect the connected components to be highly connected with the number of edges being quadratic in the number of nodes. In contrast, the set $\mathcal{V}$ corresponds to spanning trees of the connected components and, thus, the length of these lists is only linear in the number of contigs.

We observe that the time complexity is essentially linear in the number of contigs, $m$, times the cost of aligning two contigs. Additionally, we incur a cost of rejecting false positive matches of the *SWIFT* filter and a cost of maintaining the union find data structure. Let $d$ be the maximum length of a contig, $a$ be the cost of aligning two sequences, and let $\alpha(m)$ be the Ackermann function (which is known to be at most five for all practical purposes). Assuming that the contigs are random sequences, the following time complexity can be obtained when using a trivial filter that rejects two sequences if they do not share a $k$-mer.

**Lemma 1** *The time complexity of constructing $\mathcal{D}$ and $\mathcal{V}$ can be bounded by $O(m(1 + \frac{d^2}{4^k})a + \alpha(m)m)$.*

### S1.2.2 Constructing supercontigs for each set.

Similar to a partial order graph (?) or an A-Bruijn graph (?), the graph we use for constructing supercontigs has nodes that represent substrings of the contigs and directed edges for adjacencies of the substrings. We add contigs of a set $D \in \mathcal{D}$ to the graph in the order of a depth first search through the spanning tree defined by $\mathcal{V}$ (see details of partitioning step). We initialize the graph with a single node labeled with the first contig $c_1 \in D$. When adding the $l^{\text{th}}$ contig $c_l$, where $l > 1$, we enumerate all paths through the graph constructed from the $l - 1$ contigs. We locally

Table S1: Contig assembly statistics for five assembly methods.

| Method | Number of contigs | Total basepairs | N50 |
|---|---|---|---|
| *Velvet* ($k$=31) | 1166 | 244134 | 250 |
| *Velvet* ($k$=47) | 626 | 186858 | 353 |
| *Velvet* ($k$=63) | 396 | 139847 | 371 |
| *SPAdes* | 428 | 177337 | 484 |
| *MaSuRCA* | 66 | 38805 | 648 |

Figure S1: Alignment orientations distinguish four scenarios at a genomic location. Anchoring read pairs define the left end of an insertion (left) if the reference-aligned read end is in the forward orientation (blue), or the right end of the insertion (right) if the reference-aligned read end is in the reverse orientation (red). The insertion sequence is in the forward orientation with respect to the reference (top) if the two read ends align in opposite orientations, or in the reverse orientation (bottom) if they align in the same orientation.

align $c_l$ to the concatenation of substrings along each path using dynamic programming, select the path with the best alignment, and use this alignment as a guide to add $c_l$ to the graph. Depending on the begin and end position of the local alignment on the path and on $c_l$, we split or add nodes or append a prefix or suffix to labels of leaf nodes.

In detail, we first determine the position of the first and last aligned base in both $c_l$ and the path. If the alignment starts at the first position of the path, we add the prefix of $c_l$ that ends in the begin position of the alignment on $c_l$ as a prefix to the substring represented by the corresponding node. Similarly, we add a suffix to the substring represented by the last node of the path if the end position of the path equals the end position of the alignment. If the alignment does not start at the begin position of the path, but the prefix of $c_l$ that ends in the begin position of the alignment on $c_l$ has a length of at least $t$, we add a new node to the graph. Similarly, we add a new node for a suffix of $c_l$ that is at least $t$ bps long. If, in addition, the begin position of the alignment on the path falls between the begin and end of a substring represented by a node, we split the node into two and connect them by a directed edge. Similarly, we split a node if the end position of the alignment on the path falls between the begin and end of a substring represented by a node.

Adding contigs based on a single local alignment can create branching nodes but not cycles in the graph. Generally, branching nodes can have several explanations. First, the assembly of the input contigs can have errors; especially the ends of contigs tend to have low quality. Second, there may be more than one allele for the inserted sequence. And third, a part of the contigs may be repeated multiple times in the genome, although it is part of a novel sequence insertion in all cases. Motivated by the observation that ends of contigs tend to have low quality, we added new nodes to the graph only if their labels have a minimal length of $t$ (default $t = 30$). Using this parameter, we observed only very few branching cases in our test data and, thus, decided not to examine them further nor treat them specifically.

If we let $m$ be the number of contigs, $a$ be the cost of aligning a contig to a supercontig, $b_i$ be the number of paths in the component contig $i$ is inserted into and $b = \sum_i \frac{\max(b_i - 1, 0)}{m}$ then we may express the time complexity of constructing supercontigs as $O(na + nba)$. We observe that if the number of branches is small then this is linear in the number of contigs times the cost of an alignment, in the case when there are many branching components this time complexity may become prohibitive.

## S1.3 Positioning

### S1.3.1 Finding the approximate location with anchoring read pairs.

In order to identify anchoring read pairs for all contig ends, we align the unaligned reads that have the other read end aligned to the reference genome to the set of supercontigs. We rigorously filter for low quality alignments in the resulting set of anchoring read pairs and include only those with a minimal alignment score $s_{min}$ (default $s_{min} = 0.8 \cdot$ read length), at least $c_{max}$ bases not clipped (default $c_{max} = 50$), and a minimal average base call quality $q_{min}$ over each read end (default $q_{min} = 20$).

For each contig end, we cluster sets of anchoring read pairs that support the same location. Let $d_{max}$ be the maximum allowed insert size (default $d_{max} = 800$). We say that two anchoring read pairs support the same location for a contig end, if one of the read ends of each pair aligns to the contig, the other two read ends align within a distance of $d_{max}$ on the reference, the two reference aligned read ends have the same orientation, and the two contig-aligned read ends have the same orientation. We determine sets of anchoring read pairs that support the same location

by sorting them per contig by reference position, iterating over the sorted anchoring read pairs, and greedily adding each anchoring read pair to the same set as the previous if they pairwisely support the same location as the previous.

For each location supported by at least one anchoring read pair, we compute an anchoring score. This anchoring score is the number of anchoring read pairs supporting the location divided by the total number of anchoring read pairs for this contig end.

#### S1.3.2 Determining the exact position with split reads.

We consider as potential split reads all read ends that are unaligned and have the other read end aligned in the correct orientation near the insertion position. In addition, we consider read ends that align near the estimated insertion position or near the end of the contig and are clipped in the alignment.

Split read alignment algorithms that simultaneously determine the optimal split position while computing prefix and suffix alignments have previously been described, e.g. for the tools *SplazerS* (**?**) and *AGE* (**?**). We make use of the implementation in *SeqAn*.

We examine if the split alignments of our set of reads agree on a single insertion position on the reference genome. As the ends of contigs are often identical to the reference, we curate the split position to maximize the alignment to the reference. Finally, we output an insertion position for the contig end if a minimal fraction $f$ (default $f = 0.6$) of split-aligned reads support it. The split alignment further allows us to determine which subsequence of the contig is being inserted.

### S1.4 Genotyping

#### S1.4.1 Constructing alleles and read alignment.

We denote the two possible allele sequences as $R$ for the reference and $A$ for the alternate (insertion). Let $p$ be the insertion position. We construct $R$ as the subsequence of the reference genome in a window of size $2w$ around $p$ (default $w = 50$). The sequence of $A$ depends on the end that we consider of the insertion. For the left end, $A$ is the sequence from $p - w$ to $p$ on the reference genome concatenated with the first $w$ base pairs of the insertion. Similarly, when considering the right end of the insertion, we construct $A$ from the concatenation of the last $w$ base pairs of the insertion and the sequence from $p$ to $p + w$ in the reference genome.

For re-alignment, we select the set $\mathcal{R}$ of reads previously aligned to either the interval $p - w$ to $p + w$ on the reference genome or to the supercontig of the insertion. We align each read $r \in \mathcal{R}$ to both $R$ and $A$ using dynamic programming and a cost 1 for match, -4 for mismatch, -10 for gap open and -1 for gap extension, but no penalty when the read extends across the boundary of the sequence being aligned to. Only reads with alignment score at least $k$ to either $A$ or $R$ are considered for our likelihood computation. As default value we chose $k = 55$ as this is slightly larger than our window size and hence guarantees that the read considered overlaps $p$.

## S2 Preprocessing of test data

### S2.1 Simulated data

We aligned all sequencing reads of both data sets with the bwa-mem program (**?**) to the human reference genome, GRCh37 (hg19). The alignment output was realigned with the IndelRealigner from the GATK (**?**), and run through the MarkDuplicates tool of Picard[1]. From the alignment output (BAM files), we collected all read ends that were not aligned. In addition, we collected the read ends that were aligned to a different chromosome than the other read end, with a distance of 1000 or more bps to the other read end, or in discordant orientation with the other read end, and fulfilling additionally one of the following criteria: less than 50 bp matched to the reference sequence as specified by the cigar string, soft-clipping at both ends by 10 or more base pairs, or an alignment score below 50. We discard reads that were marked as optical duplicates,

[1]http://broadinstitute.github.io/picard

failed quality checks, or were supplementary alignments and refer to the resulting set of reads as unaligned reads.

Next, we further cleaned the set of unaligned reads by removing adapter sequences and discarding low quality basepairs using sickle (?) (with a minimum quality score of 20, a minimum read length of 60 bp, trimming only from the 3' end, and allowing no Ns in the reads). Only reads that passed this filtering were input to the assembly. We used *Velvet* with $k = 47$, a coverage window of $[2, 100]$, and a minimum contig length of $2k = 94$ and specified reads that have both ends unaligned as pairs and the others as single-end reads.

### S2.2 Data of 305 Icelanders

We processed the real data similar to the simulated data, but added another alignment step to exclude microbial sequences and sequences added to a newer version of the human reference. More precisely, we aligned the unaligned reads with bwa-mem (?) to a reference set of sequences that contains the sequences of GRCh38, including all alternate assemblies of GRCh38, all bacteria, the human metagenome,viruses, and UniVec adaptor sequences downloaded from NCBI[2]. Afterwards, we collected unaligned reads and proceeded as described for the simulated data.

### S2.3 Data of NA12878

We downloaded three pairs of fastq files of the Illumina Platinum genome of NA12878 (study number ERP001775, run accesion numbers ERR174324, ERR174325, and ERR174326) from the European Nucleotide Archive[3]. We aligned these 100 bp reads to GRCh38 with bwa-mem (?) and estimated the average read coverage to be 43×. We performed realignment of unaligned reads as described for the Icelandic data and collected, filtered, and assembled unaligned reads as described for the simulated data.

## S3 Supplementary results

### S3.1 Detailed analysis of results on simulated data

#### S3.1.1 Assembly results.

On the simulated chromosome 18 data sets, we obtained an average of 1582 unaligned reads per individual after alignment with bwa-mem and quality filtering with sickle (see above), and an average of 51.45 contigs per individual after assembly. Contig alignments to the simulated insertions, indicate that the assembly failed in 24.5 % of the cases when considering only a single individual. However, 90 % of the simulated insertions align to a contig of at least one individual. These 90 % are an upper bound to the recall of our approach. The other way around, we found alignments for all contigs, which implies full precision. We further examined the missing 10 insertion sequences. In all carriers of these insertions, our assembly requirements of a coverage of 2 along a minimum of 94 contiguous base pairs could not be met by the unaligned reads. Although many of the short and low frequency insertions were assembled, the missing insertions tend to have either a length just above 100 or a very low frequency appearing only as heterozygotes.

#### S3.1.2 Merging results.

The merging step reduced the set of 5154 contigs from 100 individuals to 91 supercontigs. All supercontigs align to one of the simulated insertions (using *Stellar* as above). 89 supercontigs have a one-to-one match with the set of insertions, 2 supercontigs align to different parts of the same insertion. We did not observe branching nodes in the graphs for constructing supercontigs. The quality of the contig ends is critical for determining the exact insertion position. For this

[2]ftp://ftp.ncbi.nih.gov/genomes/Bacteria/all.fna.tar.gz, Sep 20, 2013, ftp://ftp.ncbi.nih.gov/genomes/Viruses/all.fna.tar.gz, Sep 20, 2013, ftp://ftp.ncbi.nih.gov/genomes/HUMAN_MICROBIOM/Bacteria/all.fna.tar.gz, Sep 23, 2013, ftp://ftp.ncbi.nlm.nih.gov/pub/UniVec/UniVec, Jan 8, 2014

[3]http://www.ebi.ac.uk/

reason, we examined if the contigs and supercontigs contain the first and last 5 bps of each insertion sequence. Table 1 in the main text demonstrates that the merging step increases the number of fully assembled insertions by 22.7 % of all insertions. Thus, the supercontigs cover the critical ends of insertions more reliably than the original set of contigs.

#### S3.1.3 Positioning results.

After aligning the unaligned reads to the set of supercontigs, we find 280 locations on the reference sequence for the 182 ends of the supercontigs. The anchoring read pairs suggest exactly one location for 96.15 % of the contig ends, and up to 59 alternative locations for the remaining contigs. After filtering for a minimal anchoring score of 0.3, we obtain exactly one location for each end of a supercontig, which is always within an interval of 300 bps around the correct insertion position. The two supercontigs that align to different parts of the same insertion sequence anchor with a distance of 165 bps to the reference. We find sets of split reads with an unambiguous split position for 182 of the 280 unfiltered locations and 179 of the 182 filtered locations, of which 174 are correct and 5 are incorrect predictions. For 83 supercontigs we are able to determine the exact position at both ends. For the five partially assembled and one other supercontig, we find the correct position for only one end, which confirms that the quality of contig ends is critical. Our prediction is correct for three of the four ends of the two supercontigs that align to the same insertion (two true positive, one false positive, and one true negative position).

#### S3.1.4 Genotyping results.

Our genotyping algorithm genotypes 172 out of the 174 correctly positioned insert locations correctly in all 100 individuals. For two of the correctly positioned markers, the algorithm does not predict the correct genotype in all individuals. In both cases one end of the insertion is incorrectly genotyped, while the other end is correctly genotyped for all individuals. Counted per individual, *PopIns* achieves a recall of 85.4 % genotyping 5783 of the 6768 insertions correctly at both ends. Further, the algorithm predicts for all but one carriers of one insertion as heterozygous for an incorrect location of one end. This leads to an overall precision of 99 %.

## S3.2 Factors influencing running time

In many steps of *PopIns*, I/O is the primary bottleneck for the running time. These steps include finding the initially unaligned reads as well as finding anchoring read pairs for positioning contigs. The number of unaligned reads depends highly on the quality of the sequencing data, which in turn affects the amount of I/O and time needed to handle the unaligned reads (i.e. collecting mates of low-quality mapped reads, quality filtering, and assembly).

Another factor that may slow down the computations is bacterial contamination. Our implementation of *PopIns* allows to specify a reference fasta file to realign unaligned reads to known sequences before assembly. If bacterial sequences remain in the set of unaligned reads, they can lead to a considerable amount of extra contigs that cannot be placed into the human reference genome, but are input to the merging and positioning steps.

The merging step is dominated by the all-against-all comparison using the SWIFT algorithm when partitioning the contigs into sets. The running time increases with the total length of the input contigs, which is affected both by their total number and their lengths. The SWIFT parameters (k-mer size, minimum length, maximum error rate) greatly influence running time and should be chosen with care. When computing supercontigs from the computed sets, large sets may use a considerable amount of running time. Therefore, our implementation discards sets larger than ten times the number of individuals by default as they are also likely to be artifacts.

Once anchoring read pairs and potential split reads have been identified, the most time consuming task in the positioning step is the split alignment. Very high coverage at a location could lead to inacceptable running times. Hence, our implementation discards locations with a coverage greater than $cov_{max}$ (default $cov_{max} = 100$) during split alignment and also does not report an imprecise breakpoint for these locations.

Figure S2: Read alignments for three Icelanders around a 326 bp insertion (chr18:30696810, GRCh37) predicted by *PopIns*. The individuals were genotyped as homozygous carrier (top), heterozygous carrier (middle), and non-carrier (bottom). Blue reads align in the forward orientation and brown reads in the reverse complemented. Vertical yellow lines indicate mismatches with the reference genome. The insertion falls into an intron of the CCDC178 gene.

Table S2: Comparison of insertion positioning for contigs assembled from a single individual to merged supercontigs.

| | Contigs of a single individual | Merged supercontigs |
|---|---|---|
| Locations from anchoring read pairs ($a > 0.3$) | 38 | 21 |
| Pairs of locations* (both with $a > 0.3$) | 8 | 9 |
| Exact positions from split-reads | 17 | 17 |
| Pairs of positions* from split-reads | 4 | 7 |

* for the two ends of the same contig

## S3.3 Performance of *PopIns* on a single individual

We positioned the contigs assembled from one of the 305 Icelandic individual (sequenced at a coverage of 23.6×) without applying the merging step and contigs assembled from the NA12878 data described in Sect. S2.3.

### S3.3.1 Single individual versus multiple individuals.

In order to quantify the benefit from the merging step on real data, we used the contigs from an Icelandic individual and compared it to all supercontigs into which the individual's contigs were merged. Table S2 shows the number of locations and exact positions predicted on chromosome 18. These numbers confirm that the merging step improves the quality of the sequences and, thus, our ability to find an unambiguous position. In addition, it suggests that filtering by anchoring score using anchoring read pairs from all individuals in comparison to one individual, identifies locations with higher precision.

### S3.3.2 Insertions for the individual NA12878.

We ran the assembly, positioning, and genotyping step of *PopIns* on the data from the individual NA12878. *PopIns* identifies 213 insertions in full length with precise breakpoints for both ends that are less than 50 bp apart and genotyped as both heterozygote or both homozygote. These insertions have lengths between 63 and 3584 bps with a median length of 230 bp and a mean length of 454 bp.

If we include assembled contigs where only one end of the assembled sequence can be positioned with a precise breakpoint, *PopIns* predicts 1246 insertion ends genotyped as heterozygous or homozygous. Further including contig ends without precise breakpoints yields 3127 positions (before genotyping) each supported by at least 3 anchoring read pairs and an anchoring score above 0.3.

### S3.3.3 Comparison to validated insertions of NA12878.

We downloaded a data set of 74 insertions derived from fosmid clones of NA12878 (**?**). 30 of these insertions have additionally been valided (**?**). We selected the 61 of these 74 insertions that are annotated as novel sequence insertions and obtained a mean and median length of 5.1 kb. Converting their positions from GRCh36 (hg18) to GRCh38 using the liftover tool further reduced the set to 57 insertions. We compared them to the positions predicted by *PopIns* allowing a shift of up to 150 bp in both directions.

Given the lengths of the insertions in this set, the approach implemented in *PopIns* is likely to fail on a single individual during the assembly step. Still, *PopIns* predicts the positions of both ends correctly for 6 insertions and one end for an additional 6 insertions. Of these, we find split reads on both ends of 3 insertions and on one end of 5 insertions. For one insertion, *PopIns* assembles the full length sequence correctly.

#### S3.3.4 Comparison to novel sequence insertions of NA12878 from 1000 genomes project.

A set of 111 novel sequence insertions is available from the 1000 genomes project[4] (**?**). Of these, we selected the 51 insertions that have a length longer than 100 bp. They have an average length of 558 bp and a median length of 215 bp and were discovered with the tools Cortex (**?**), SOAP (**?**), and NovelSeq (**?**). For 20 of the 51 insertions, of which 18 were detected by NovelSeq and 2 by Cortex, the vcf file specifies a confidence interval of up to 185 bp. Therefore, we allowed a difference of up to 200 bp between insertion positions when comparing them to the output of *PopIns*. Again, we converted the 1000 genomes positions from GRCh36 (hg18) to GRCh38 prior to comparison and confirmed that none of the positions had been updated in the newer version of the reference genome.

*PopIns* is able to find a total of 29 of these insertions: 24 of the insertions are found in full length, both ends with different contigs are found for an additional 3 insertions, and one end is found for an additional 2 insertions. When splitting by tools, *PopIns* detects at least one end of 22 of 26 insertions predicted by Cortex, 7 of 9 insertions predicted by SOAP, and 4 of 20 insertions predicted by NovelSeq. The numbers include 4 insertions detected by two or more tools. This shows that the agreement of *PopIns* with Cortex and SOAP is high although *PopIns* implements a less time consuming approach. We do not know whether the low agreement with NovelSeq is due to the specified confidence intervals. For all but two of all recovered positions, *PopIns* finds split reads.

[4] ftp://ftp.1000genomes.ebi.ac.uk/vol1/ftp/pilot_data/paper_data_sets/ companion_papers/mapping_structural_variation/
